# Supplementary material for: Suppressors of selection
Source: arXiv:1607.04469 source file (2016-12-20)
Supplement: Supplementary file 1 [file SupportingInformation.pdf]

# Supporting Information

As supplementary information, we include here the text of the SageMath program which we ran

- to compute the exact fixation probability $\Phi(r)$ for the graphs $\ell_6$, $\ell_8$ and $\ell_{10}$ when the fitness values $r \in \{1, \ldots, d+1, 1/2, \ldots, 1/d\}$,
- to solve the linear system

$$\sum_{i=0}^{d} a_i r^i = \Phi(r) \left( \sum_{i=0}^{d} b_i r^i \right),$$

where $\Phi'(r) = \sum_{i=0}^{d} a_i r^i$ and $\Phi''(r) = \sum_{i=0}^{d} b_i r^i$ are the numerator and the denominator of the rational function $\Phi(r)$. The symmetries of the graph allow to reduce the degree which is now bounded by $d = \frac{N(N+1)}{2} - 2 \ll 2^N - 2$. Next, we give the exact values of $\Phi = \Phi'/\Phi''$ and $\Delta = \Delta'/\Delta''$ for the graphs $\ell_6$, $\ell_8$ and $\ell_{10}$.

## Text of the SageMath program

```
#
# The l-family checker
#
# The graph l_{2n+2} is a complete graph K_{2n} with two more nodes
# each of them connected with half the nodes of the complete core.
# These new nodes are also joint by an edge.
#
# The nodes are writen as
#
#       (e,k,k',e')
#
# where e,e'\in\{0,1\} represents if the external nodes are mutants or not,
# and k,k'\in{0,1,...,n} the number of mutants of each halves of the complete
# core. Using the symmetries of the graph, it is possible to reduce the nodes
# to those with (lexicographically)
#
#       k >= k'                 e >= e'
#

# The parameter n is:
n = 2 # change it to 3 and 4 to reproduce the results of the paper



#
# Reduces the state s to a canonical form
#
def reduce_state(s):
    if s[1] < s[2]:
        return (s[3],s[2],s[1],s[0])
    if (s[1] == s[2]) and (s[3] > s[0]):
        return (s[3],s[2],s[1],s[0])
    return s
```

```
#
# Computes the possible (reduced) states for a given n, it returns the list of
# states and the position of the states in the list
#
def ComputeStates(n):
    # Compute the states
    states = []
    for k in [0..n]:
        for kp in [0..k]:
            if k != kp:
                states.extend([ (0,k,kp,0), (1,k,kp,0), (0,k,kp,1), (1,k,kp,1) ])
            else:
                states.extend([ (1,k,kp,1), (1,k,kp,0), (0,k,kp,0) ])

    istates = { v:k for k,v in enumerate(states)}

    s0 = states[0]
    sn = states[-1]
    states[0] = (0,0,0,0)
    states[-1] = (1,n,n,1)
    states[istates[(0,0,0,0)]] = s0
    states[istates[(1,n,n,1)]] = sn
    istates[s0] = istates[(0,0,0,0)]
    istates[sn] = istates[(1,n,n,1)]
    istates[(0,0,0,0)] = 0
    istates[(1,n,n,1)] = len(states)-1
    return states, istates


#
# Computes the matrix P and the vector b for the list
#
def ComputePb(r,n,states,istates):

    # Compute matrix
    P = matrix(PP,[[0]*len(states)]*len(states) )

    for s in states:
        m = sum(s)
        P[istates[s],istates[s]] = r * m + 2 * n + 2 - m


    for s in states:
        # Leftmost
        if s[0] == 1:
            P[istates[s],istates[(1,s[1],s[2],1)]] -= r/(n+1)
```

```
    if s[1] == n:
        P[istates[s],istates[s]] -= r*n/(n+1)
    else:
        P[istates[s],istates[(s[0],s[1]+1,s[2],s[3])]] -= r*(n-s[1])/(n+1)
        P[istates[s],istates[s]] -= r*s[1]/(n+1)
else:
    P[istates[s],istates[(0,s[1],s[2],0)]] -= 1/(n+1)

    if s[1] == 0:
        P[istates[s],istates[s]] -= n/(n+1)
    else:
        P[istates[s],istates[reduce_state((s[0],s[1]-1,s[2],s[3]))]] -= s[1]/(n+1)
        P[istates[s],istates[s]] -= (n-s[1])/(n+1)

# Rightmost
if s[3] == 1:
    P[istates[s],istates[(1,s[1],s[2],1)]] -= r/(n+1)
    if s[2] == n:
        P[istates[s],istates[s]] -= r*n/(n+1)
    else:
        P[istates[s],istates[reduce_state((s[0],s[1],s[2]+1,s[3]))]] -= r*(n-s[2])/(n+1)
        P[istates[s],istates[s]] -= r*s[2]/(n+1)
else:
    P[istates[s], istates[(0,s[1],s[2],0)]] -= 1/(n+1)

    if s[2] == 0:
        P[istates[s],istates[s]] -= n/(n+1)
    else:
        P[istates[s],istates[(s[0],s[1],s[2]-1,s[3])]] -= s[2]/(n+1)
        P[istates[s],istates[s]] -= (n-s[2])/(n+1)



# Core left
if s[1] == n:
    P[istates[s],istates[(1,n,s[2],s[3])]] -= r/2
    P[istates[s],istates[s]] -= r*(n-1)/2
    if s[2] == n:
        P[istates[s],istates[s]] -= r*n/2
    else:
        P[istates[s],istates[reduce_state((s[0],n,s[2]+1,s[3]))]] -= r*(n-s[2])/2
        P[istates[s],istates[s]] -= r*s[2]/2
elif s[1] == 0:
    P[istates[s],istates[(s[3],0,0,0)]] -= 1/2
    P[istates[s],istates[s]] -= (n-1)/2 + n/2
else:
    P[istates[s],istates[(1,s[1],s[2],s[3])]] -= s[1]*r/(2*n)
    P[istates[s],istates[reduce_state((0,s[1],s[2],s[3]))]] -= (n-s[1])/(2*n)
    P[istates[s],istates[s]] -= s[1]*r*(s[1]-1)/(2*n) + (n-s[1])*(n-s[1]-1)/(2*n)
```

```
            P[istates[s],istates[(s[0],s[1]+1,s[2],s[3])]] -= s[1]*r*(n-s[1])/(2*n)
            P[istates[s],istates[reduce_state((s[0],s[1]-1,s[2],s[3]))]] -= (n-s[1])*s[1]/(2*n)
            P[istates[s],istates[s]] -= r*s[1]*s[2]/(2*n) + (n-s[1])*(n-s[2])/(2*n)
            P[istates[s],istates[reduce_state((s[0],s[1],s[2]+1,s[3]))]] -= r*s[1]*(n-s[2])/(2*n)

            if s[2] != 0:
                P[istates[s],istates[(s[0],s[1],s[2]-1,s[3])]] -= (n-s[1])*s[2]/(2*n)

        # Core right
        if s[2] == n:
            P[istates[s],istates[(1,n,n,s[0])]] -= r/2
            P[istates[s],istates[s]] -= r*(2*n-1)/2
        elif s[2] == 0:
            P[istates[s],istates[(s[0],s[1],0,0)]] -= 1/2

            if s[1] == 0:
                P[istates[s],istates[s]] -= (2*n-1)/2
            else:
                P[istates[s],istates[s]] -= (n-1)/2 + (n-s[1])/2
                P[istates[s],istates[reduce_state((s[0],s[1]-1,0,s[3]))]] -= s[1]/2
        else:
            P[istates[s],istates[reduce_state((s[0],s[1],s[2],1))]] -= s[2]*r/(2*n)
            P[istates[s],istates[(s[0],s[1],s[2],0)]] -= (n-s[2])/(2*n)
            P[istates[s],istates[s]] -= s[2]*r*(s[2]-1)/(2*n) + (n-s[2])*(n-s[2]-1)/(2*n)
            P[istates[s],istates[s]] -= r*s[2]*s[1]/(2*n) + (n-s[2])*(n-s[1])/(2*n)
            P[istates[s],istates[reduce_state((s[0],s[1],s[2]+1,s[3]))]] -= s[2]*r*(n-s[2])/(2*n)
            P[istates[s],istates[(s[0],s[1],s[2]-1,s[3])]] -= (n-s[2])*s[2]/(2*n)
            if s[1] != n:
                P[istates[s],istates[(s[0],s[1]+1,s[2],s[3])]] -= r*s[2]*(n-s[1])/(2*n)
            P[istates[s],istates[reduce_state((s[0],s[1]-1,s[2],s[3]))]] -= (n-s[2])*s[1]/(2*n)

    b=-P[1:len(states)-1,len(states)-1]
    P=P[1:len(states)-1,1:len(states)-1]
    return P,b


#
# Computes the average fixation probability function
#
def Phi(P,b,n,istates):
    sol = P.solve_right(b)
    return sol[istates[(1,0,0,0)]-1,0] / (n + 1) + sol[istates[(0,1,0,0)]-1,0] * n / (n + 1)


#
# "Entry point"
#
```

```
# Computes the states for the given size
states, istates = ComputeStates(n)

# A first estimate of the degree of the rational function Phi
num_fac = len(states) - 2
fits=[1..num_fac+1]
fits.extend([ 1/f for f in fits[1:-1] ])

# Compute the fixation probabilities for the selected fitnesses
fps = {
    f : Phi(*ComputePb(f, n, states, istates), n=n, istates=istates)
    for f in fits
}

# Now we are ready to compute the coefficients of the function.
# Construct the matrix of the linear system describing the function \Phi
X = matrix(PP, [[1]*len(fits)]*len(fits) )
X[:,num_fac-2] = [ [r] for r in fits ]
X[:,-1] = [ [ -fps[r] ] for r in fits ]
X[:,-2] = [ [ -r*fps[r] ] for r in fits ]

y = vector(PP, [(fps[r]-1)*r**num_fac for r in fits ] )

for i in xrange(num_fac-3,-1,-1):
    X[:,i] = X[:,i+1].elementwise_product( X[:,num_fac-2] )
    X[:,num_fac + i] = X[:,num_fac+i+1].elementwise_product( X[:,num_fac-2] )

# Solve it
sol = X.solve_right(y)

# Create the field of fuctions. Then x is regarded as the variable of the
# field P(x). You can bypass this step to simplify later the expressions
# (that is regarding x as a symbolic variable with no special meaning)
F.<x> = Frac(PP['x'])

# Construct the function
FB = (sum( sol[num_fac-1-i]* x**i for i in [0..num_fac-1] ) + x**num_fac) / \
                     (sum( sol[-(i+1)]* x**i for i in [0..num_fac-1] ) + x**num_fac)
pretty_print(FB)

# and finally the Delta
Delta = FB - x**(2*n+1)/sum( x**i for i in range(2*n+2) )
pretty_print(Delta)

# take a look to the numerator and denominator
pretty_print(Delta.denominator())
pretty_print(Delta.numerator()/(x-1)) # up to (x-1)
```

## Graph $\ell_6$

$$\Phi'(r) = r^{17} + \frac{20010803101}{2356885440}r^{16} + \frac{12872954057}{368903808}r^{15} + \frac{146529682470259}{1590897672000}r^{14} + \frac{20006411662050293}{114544632384000}r^{13} + \frac{57705463723529081}{229089264768000}r^{12} + \frac{9771555843017869}{34363389715200}r^{11} + \frac{1025122250624863}{4042751731200}r^{10} + \frac{60836752923313811}{343633897152000}r^{9} + \frac{9233243223215201}{98181113472000}r^{8} + \frac{1542392404026107}{42954237144000}r^{7} + \frac{3153322564729}{357951976200}r^{6} + \frac{496442293}{474304896}r^{5}$$

$$\Phi''(r) = r^{17} + \frac{22367688541}{2356885440}r^{16} + \frac{1883112090533}{42423937920}r^{15} + \frac{579196292648299}{4242393792000}r^{14} + \frac{23779172425823219}{76363088256000}r^{13} + \frac{17230349794290811}{30545235302400}r^{12} + \frac{55592085032472109}{65454075648000}r^{11} + \frac{71798191286820983}{65454075648000}r^{10} + \frac{37885437915832519}{30545235302400}r^{9} + \frac{37885437915832519}{30545235302400}r^{8} + \frac{71798191286820983}{65454075648000}r^{7} + \frac{55592085032472109}{65454075648000}r^{6} + \frac{17230349794290811}{30545235302400}r^{5} + \frac{23779172425823219}{76363088256000}r^{4} + \frac{579196292648299}{4242393792000}r^{3} + \frac{1883112090533}{42423937920}r^{2} + \frac{22367688541}{2356885440}r + 1$$

$$\Delta'(r) = r^5(r-1)(-\frac{1}{408}r^{13} - \frac{17959403797}{509087255040}r^{12} - \frac{2269495014623}{9163570590720}r^{11} - \frac{165933379973713}{152726176512000}r^{10} - \frac{4365681088426001}{1374535588608000}r^{9} - \frac{4487811876686051}{687267794304000}r^{8} - \frac{6774104367192077}{687267794304000}r^{7} - \frac{673669214287879}{59762416896000}r^{6} - \frac{13704670736178649}{1374535588608000}r^{5} - \frac{2361661570426121}{343633897152000}r^{4} - \frac{2506212053017441}{687267794304000}r^{3} - \frac{122207986609099}{85908474288000}r^{2} - \frac{299174081287}{818175945600}r^{1} - \frac{22137397}{474304896})$$

$$\Delta''(r) = r^{21} + \frac{22367688541}{2356885440}r^{20} + \frac{1925536028453}{42423937920}r^{19} + \frac{619458132022099}{4242393792000}r^{18} + \frac{27245137277038619}{76363088256000}r^{17} + \frac{15493177389178517}{21818025216000}r^{16} + \frac{552157240360000477}{458178529536000}r^{15} + \frac{411797892764062669}{229089264768000}r^{14} + \frac{550050599259865931}{229089264768000}r^{13} + \frac{1329324154659596831}{458178529536000}r^{12} + \frac{54074574184168127}{16969575168000}r^{11} + \frac{54074574184168127}{16969575168000}r^{10} + \frac{1329324154659596831}{458178529536000}r^{9} + \frac{550050599259865931}{229089264768000}r^{8} + \frac{411797892764062669}{229089264768000}r^{7} + \frac{552157240360000477}{458178529536000}r^{6} + \frac{15493177389178517}{21818025216000}r^{5} + \frac{27245137277038619}{76363088256000}r^{4} + \frac{619458132022099}{4242393792000}r^{3} + \frac{1925536028453}{42423937920}r^{2} + \frac{22367688541}{2356885440}r + 1$$

## Graph $\ell_8$

$$\Phi'(r) = r^{31} + \frac{134280899640541}{8309364148800}r^{30} + \frac{51436353602527862867}{399248328621542400}r^{29} + \frac{261395239481852545538087881}{387350728428620436480000}r^{28} + \frac{58380787959652779590779931453}{223695045667528302067200000}r^{27} + \frac{2732442855095140200328064602 87}{344146224103889695488000000}r^{26} + \frac{10954679493630837091790247744 9001}{55418643571826366447616000000}r^{25} + \frac{1038203195769664571995777599649}{25100123467406200012800000}r^{24} + \frac{9219730675269628384323897931 1641}{12437849417025284053401600000}r^{23} + \frac{11740712284825831069430912101427861}{10180610078379954725191680000 0}r^{22} + \frac{10329379523929482321277816205081 11}{65681355344386804678656000000}r^{21} + \frac{2080310449462551016365104268144504161}{109950588846503511032070144000 00}r^{20} + \frac{753897025982731385467385013243433}{373981594715998336843776 0000}r^{19} + \frac{2463546677977027065113743507694 3581}{12935363393706295415537664000 0}r^{18} + \frac{12515631613942324399852954221 13577}{785361348903596507371929600 0}r^{17} + \frac{3477901185411691168774411224802753}{2955660990497406210539520000 0}r^{16} + \frac{5510437720885200677122578161372417}{7233591371480494146846720000 0}r^{15} + \frac{4709031129091755423187995718697467 73}{109950588846503511032070144000 00}r^{14} + \frac{5969238263774975752904624513257 19}{2893436548592197658738688000 0}r^{13} + \frac{7066876349108602065069037131219649}{8457737603577193156313088000 00}r^{12} + \frac{15230658652580143385602731564041827}{54975294423251755516035072000 00}r^{11} + \frac{1419300274241719705184148447121 31}{1963403372258991268429824000 00}r^{10} + \frac{9117450368110736467921341657 73}{654467790752997089476608000 0}r^{9} + \frac{6249152838837548879426501}{354149237420452970496000}r^{8} + \frac{11363885694605603}{10303182674104320}r^{7}$$

$$\Phi''(r) = r^{31} + \frac{142590263789341}{8309364148800}r^{30} + \frac{685751104869983351}{4697039160253440}r^{29} + \frac{317970272348671658719761481}{387350728428620436480000}r^{28} + \frac{614045446315686238195542724177}{178956036534022641653760000}r^{27} + \frac{782883035835001850913227050807}{68829244820777939097600000}r^{26} + \frac{2027468204090641240495620587659}{65074922376008233328640000}r^{25} + \frac{6233679485365536931871855089022867}{85898897536330867993804800000}r^{24} + \frac{5405997383885275954244381013403073}{36813813229856086283059200000}r^{23} + \frac{5412233502300397035053907892438 4011}{206157354087194083185131520000}r^{22} + \frac{17335457980981817006013641394207246 67}{412314708174388166370263040000 0}r^{21} + \frac{1677617314994594652141277695694600403}{2748764721162587775801753600000}r^{20} + \frac{1337864897706719539236595661589558203}{1649258832697552665481052160000}r^{19} + \frac{1066417788134171727139974541494 04519}{1070947293959449782779904000 00}r^{18} + \frac{9374593978090858152054746159000953163}{8246294163487763327405260800000}r^{17} + \frac{3969636168792774061518691713246829 3}{3272338953764985447383040000 0}r^{16} + \frac{39696361687927740615186917132468293}{32723389537649854473830400000}r^{15} + \frac{9374593978090858152054746159000953163}{8246294163487763327405260800000}r^{14} + \frac{106641778813417172713997454149404519}{107094729395944978277990400000}r^{13} + \frac{1337864897706719539236595661589558203}{1649258832697552665481052160000}r^{12} + \frac{1677617314994594652141277695694600403}{2748764721162587775801753600000}r^{11} + \frac{173354579809818170060136413942072 4667}{412314708174388166370263040000 0}r^{10} + \frac{54122335023003970350539078924384011}{206157354087194083185131520000}r^{9} + \frac{5405997383885275954244381013403073}{36813813229856086283059200000}r^{8} + \frac{6233679485365536931871855089022867}{85898897536330867993804800000}r^{7} + \frac{2027468204090641240495620587659}{65074922376008233328640000}r^{6} + \frac{782883035835001850913227050807}{68829244820777939097600000}r^{5} +$$

$$\frac{614045446315686238195542724177}{17895603653402264165376000}r^4 + \frac{317970272348671658719761481}{387350728428620436480000}r^3 +$$
$$\frac{685751104869983351}{4697039160253440}r^2 + \frac{142590263789341}{8309364148800}r + 1$$

$$\Delta'(r) = r^7(r-1)(-\frac{1}{304}r^{27} - \frac{25197109151333}{398849479142400}r^{26} -$$
$$\frac{79418092024874684869}{1306630893670502400000}r^{25} - \frac{1514393785629240226219612 9}{387350728428620436480000}r^{24} -$$
$$\frac{2366973910210561053038186471}{124943850961935807990988800}r^{23} - \frac{845531429520747906230096887311 1}{114531863381774490658406400000}r^{22} -$$
$$\frac{991524478799860112838020328209849}{4123147081743881663702630400000}r^{21} - \frac{5521164844468759159410730585869037}{8246294163487763327405260800000}r^{20} -$$
$$\frac{985364585564805190812437620862539}{610836604702797283511500800000}r^{19} - \frac{111731529120083126099350945280644519}{32985176653951053309621043200000}r^{18} -$$
$$\frac{2054609370880573116532051768359613 21}{32985176653951053309621043200000}r^{17} - \frac{1107344936703037327615550011157875 13}{109950588846503511032070144000000}r^{16} -$$
$$\frac{158032724138319990637134255263110231}{10995058884650351103207014400000}r^{15} - \frac{199802720995875508460288885619407237}{10995058884650351103207014400000}r^{14} -$$
$$\frac{224538609583176412587468836353029011}{10995058884650351103207014400000}r^{13} - \frac{24094663993232446388630691852040643}{1178042023355394761057894400000}r^{12} -$$
$$\frac{150767863647126646217505642437799077}{8246294163487763327405260800000}r^{11} - \frac{53451052002645000374177015848862851}{3665019628216783701069004800000}r^{10} -$$
$$\frac{341577973854758089828094884500692837}{32985176653951053309621043200000}r^9 - \frac{61349821821294974981199564322522 81}{9424336186843158088463155200000}r^8 -$$
$$\frac{56390563795674089013546736289013 77}{1570722697807193014743859200000}r^7 - \frac{18840773531540731523638914353570237}{10995058884650351103207014400000}r^6 -$$
$$\frac{21810108918165622062295652917 1233}{314144539561438602948771840000}r^5 - \frac{85136118048946532310061747931273}{366501962821678370106900480000}r^4 -$$
$$\frac{132994911304258723701851574251}{215758612336152886640640000 0}r^3 - \frac{796217688916573522810090562 53}{6544677907529970894766080000}r^2 -$$
$$\frac{5624933677952289415541 81}{354149237420452970496000}r - \frac{1060703020501283}{10303182674104320})$$

$$\Delta''(r) = r^{37} + \frac{142590263789341}{8309364148800}r^{36} + \frac{690448144030236791}{4697039160253440}r^{35} +$$
$$\frac{324617284268784317447995081}{387350728428620436480000}r^{34} + \frac{640351350752994828494392138177}{17895603653402264165376000 0}r^{33} +$$
$$\frac{109273453925159158351768202976 01}{894780182670113208268800000}r^{32} + \frac{306957477135913987153449321197}{88373351374825995878400 00}r^{31} +$$
$$\frac{348454767609907409188939226679 07}{410999509743209894707200000}r^{30} + \frac{467926040237875745525012678855260 31}{2576966926089926039814144 00000}r^{29} +$$
$$\frac{511409203336033971112694965250569 73}{14725525291942434513223680 0000}r^{28} + \frac{827208499195876349134187545906993721}{13743823605812938879008768 00000}r^{27} +$$
$$\frac{788997422725635421765930623910844 1937}{8246294163487763327405260800000}r^{26} + \frac{116242802695426289691320529746596 77181}{8246294163487763327405260800000}r^{25} +$$
$$\frac{190566613632525673986701170263208391}{9817016861294956342149120 0000}r^{24} + \frac{785680055939815191787545230787594 01}{3123596274048395199774720 0000}r^{23} +$$
$$\frac{105886022749561898768542930545605 4977}{3435955901453234719752192 00000}r^{22} + \frac{738362330204465247111688896579305 0837}{2061573540871940831851315 200000}r^{21} +$$
$$\frac{171696558089818710749913085963004 8009}{4340154822888296488108032 00000}r^{20} + \frac{342788185806153687822426315538349 01977}{8246294163487763327405260800000}r^{19} +$$
$$\frac{342788185806153687822426315538349 01977}{8246294163487763327405260800000}r^{18} + \frac{171696558089818710749913085963004 8009}{4340154822888296488108032 00000}r^{17} +$$
$$\frac{738362330204465247111688896579305 0837}{2061573540871940831851315 200000}r^{16} + \frac{105886022749561898768542930545605 4977}{3435955901453234719752192 00000}r^{15} +$$
$$\frac{785680055939815191787545230787594 01}{3123596274048395199774720 0000}r^{14} + \frac{190566613632525673986701170263208391}{9817016861294956342149120 0000}r^{13} +$$
$$\frac{116242802695426289691320529746596 77181}{8246294163487763327405260800000}r^{12} + \frac{788997422725635421765930623910844 1937}{8246294163487763327405260800000}r^{11} +$$
$$\frac{827208499195876349134187545906993721}{13743823605812938879008768 00000}r^{10} + \frac{511409203336033971112694965250569 73}{14725525291942434513223680 0000}r^9 +$$
$$\frac{467926040237875745525012678855260 31}{2576966926089926039814144 00000}r^8 + \frac{348454767609907409188939226679 07}{410999509743209894707200000}r^7 +$$
$$\frac{306957477135913987153449321197}{88373351374825995878400 00}r^6 + \frac{109273453925159158351768202976 01}{894780182670113208268800000}r^5 +$$
$$\frac{640351350752994828494392138177}{17895603653402264165376000 0}r^4 + \frac{324617284268784317447995081}{387350728428620436480000}r^3 +$$
$$\frac{690448144030236791}{4697039160253440}r^2 + \frac{142590263789341}{8309364148800}r + 1$$

**Graph $\ell_{10}$**

$$\Phi'(r) = r^{49} + \frac{63998337467225103992090545275949}{2453784351049966935520268248500} r^{48} +$$
$$\frac{1467791915119732826876236247120465601078713}{4347173063939489764811377306367332725000} r^{47} +$$
$$\frac{35863545786298851175250332766194774847587066497001}{12401832675459773375542137748470045164516250000} r^{46} +$$
$$\frac{10107225020718561540118243112729380257297990160772275379}{548483451904883937306726584063836217445895672500000} r^{45} +$$
$$\frac{17397736112593212118849985482353558760254598400369231894071}{186745556243805721511575956002687093082769240875000000} r^{44} +$$
$$\frac{1584820175953684739314764508568609751473509134206333820165933161}{4072981476967482288033181896925997680709028481279687500000} r^{43} +$$
$$\frac{5172744630351475138604328343512155631419526181205299637199565311977}{3747142958810083704990527345171917866252306202777312500000000} r^{42} +$$
$$\frac{4952120295598135430003008711918788531699356080751711979186627645861149}{1166544768492718163948366802457468114678020588917252812500000000} r^{41} +$$
$$\frac{232819629505635204261122698697497213530179530184438758651042497936165479}{202621861840806084073867442740280375889036785127231785156250000000} r^{40} +$$
$$\frac{140705161942293599314085668376462617712634457962573176050687488215725213}{507881210001272264607149968709269928341394111617079296875000000} r^{39} +$$
$$\frac{704776109036054971829235346720766616789810509486535754147964424687649474571}{11732055951029389312425164277184135344686203978354531757812500000000} r^{38} +$$
$$\frac{560923897879890207748212897673461209350427363232082881495578421471399410965213}{47514826601669026715321915322595748145979126112335853619140625000000000} r^{37} +$$
$$\frac{502667498451061439286536771249640753000401734211654584203734622109856518280909}{23757413300834513357660957661297874072989563056167926809570312500000000} r^{36} +$$
$$\frac{2642982401545335688749171370572651127697436882617726500323253117106612145203}{76023722562670442744515064516153197033566601779737365790625000000000} r^{35} +$$
$$\frac{20823387297836818281526008435918371919883630252711427765368887472917082446989053}{3959568883472418892943492943549645678831593842694654468261718750000000000} r^{34} +$$
$$\frac{218249476472181748593498178533365602635257369680047412113593696562977826835140353}{29696766626043141697076197076622342591236953820209908511962890625000000000} r^{33} +$$
$$\frac{12073616682732932701560441487145827994410542880111327873960403995706625725384629}{12690925908565445169690682511377069483434595649662354064941406250000000000} r^{32} +$$
$$\frac{135789940566315840585532565857821740547661945056372353589849669605940440768457227}{118787066504172566788304788306489370364947815280839634047851562500000000000} r^{31} +$$
$$\frac{1263938665010845091528254131320795020467290201523310371883484596474040356624342127}{9898922208681047232358732358874114197078984606736636170654296875000000000} r^{30} +$$
$$\frac{3893768339258599798434728937074950725159562999271918086462520859044296962887753}{2934463105340231392991719078717622785695351168004931671142578125000000} r^{29} +$$
$$\frac{1216824486353361237463418998567150903579908174072483322171283158910558540587207}{948172625352590731068844095677597145314078985319601165771484375000000} r^{28} +$$
$$\frac{342950658867614575564774744874331500786589425104481846989084698332117314061325299}{29696766626043141697076197076622342591236953820209908511962890625000000000} r^{27} +$$
$$\frac{136620889917538222852217823124817295526976539096842805176370201484115198050916799}{14141317440972924617655331941248734567255692295338051672363281250000000000} r^{26} +$$
$$\frac{106103728708961707725096565755154094753809519630524214452593627351709782825503313}{14141317440972924617655331941248734567255692295338051672363281250000000000} r^{25} +$$
$$\frac{496044793580204554525678229969923834502352531064764912680884504837714700470547}{918835601053315027756070454103414065322925551367880832672119140625000} r^{24} +$$
$$\frac{772359485654188724829120426699784984692635338460009360833608747322067262809039}{2151939610582836354860593991059590042843257523203616558837890625000000} r^{23} +$$
$$\frac{652516365227989567609612927273551680629147392704119960328347885247676692854839209}{29696766626043141697076197076622342591236953820209908511962890625000000000} r^{22} +$$
$$\frac{366302474000671446200946961697442757335305613890313285591333774174703031631539261}{29696766626043141697076197076622342591236953820209908511962890625000000000} r^{21} +$$
$$\frac{1645494418668165225995421450087912710711608999941997419463709015853368829896609}{2604979528600275587462824304966872157126048580720167413330078125000000000} r^{20} +$$
$$\frac{3483355672276308965948183203469013565617881463433844672444674298813595385516279}{1187870665041725667883047883064893703649478152808396340478515625000000000} r^{19} +$$
$$\frac{36366071775932414505549205751279497624573418272160719024002888028025852967255521}{29696766626043141697076197076622342591236953820209908511962890625000000000} r^{18} +$$
$$\frac{1566098453886886032512195177922507302933744244599563429255680654923560486349}{343712576690314140012455984683128965176353632178355422592163085937500} r^{17} +$$
$$\frac{9849998529036909725835193690470491230633425936733439335488624857067513903961}{6599281472454031488239154905916076131385989737824424113769531250000000} r^{16} +$$
$$\frac{7612244671643394966002495975771535194184958698344817283774206365930539589}{179572284964735550700385167507920438949278632321753037109375000000000} r^{15} +$$
$$\frac{1780331892413176694593527982155770314406131540035651123394684892300797027}{174046983888897533755757931584599810058531597481083712890625000000000} r^{14} +$$
$$\frac{666823956195516846359952872220117109274829807880728490758393042227}{3269408920614211209838601138059543722335523574360546875000000000} r^{13} +$$
$$\frac{502416727669024719925142702253603868291369674070233164892842561}{155686139076867200468504816098073510587405884493359375000000} r^{12} +$$
$$\frac{20309000357168189131016179693765660499567247658979879117}{53446944490858694730872157429537304821434882812500000} r^{11} +$$
$$\frac{2231094028186541795006656736377928879201619060106379}{75358358271022928497217850902161732770498046875000} r^{10} +$$
$$\frac{2160930461505967730083659877408854787}{1886943135237232727224847699296875000} r^{9}$$

$$
\begin{aligned}
\Phi''(r) = r^{49} + \frac{66452121818275070927610813524449}{2453784351049966935520268248500} r^{48} + \\
\frac{3171065904103137883917151919165713711668601}{8694346127878979529622754612734665450000} r^{47} + \\
\frac{161551466808961078632134160985357629261818985772279}{49607330701839093502168550993880180658065000000} r^{46} + \\
\frac{2068529647022090441678077299141302609199588004130495071}{95388426418240684748995927663275863903634030000000} r^{45} + \\
\frac{450435638313535005425039251624357069084344950220101681650037}{3921656681119920151743095076056428954738154058375000000} r^{44} + \\
\frac{6867963997466308046319209185518123663135600673726493180976212363}{13625974395673031654511008527897883150008386191917500000000} r^{43} + \\
\frac{269061418914533471263783319921967679903930817801083532938975715087}{142748303192765093523448660768454013952468807724850000000000} r^{42} + \\
\frac{10872394332592777284288878621556700840415990768352322461450204898552609}{17731480481089316092015175397353515343105912951542242750000000000} r^{41} + \\
\frac{38291101140138887359782676914615116290259958340221391656013420168256811577}{21721063589334412212718589861758056295304743365639247368750000000000} r^{40} + \\
\frac{98514958000354677455643814676264534931115549410475725682221654907248284623}{21721063589334412212718589861758056295304743365639247368750000000000} r^{39} + \\
\frac{26732729318515826831791274995616579065637953912223549102534868243984792082723}{2534124085422348091483835483871773234452220059324578859687500000000000} r^{38} + \\
\frac{425183741527331139825902027524200329764363303966235727482073723400678572174677}{190059306406676106861287661290382992583916504449343414476562500000000000} r^{37} + \\
\frac{828072648510561263189682099297410898323565661136075420452698337442115035231749}{190059306406676106861287661290382992583916504449343414476562500000000000} r^{36} + \\
\frac{14904297300954246434065316373615468433612748954602965427264845089050815525174899}{1900593064066761068612876612903829925839165044493434144765625000000000000} r^{35} + \\
\frac{41550484881909446388327767743277061617985477251726998056709651669094404010048507}{3167655106777935114354794354839716543065275074155723574609375000000000000} r^{34} + \\
\frac{22130456707641639004248146630609315027823814070629995136603247025845612921651603}{1079882422765205152620952620968085185135889229825814854980468750000000000} r^{33} + \\
\frac{1784422236438075188537138900658095059296529954702208506947548731323074538577597981}{593935332520862833941523941532446851824739076404198170239257812500000000000} r^{32} + \\
\frac{3287151019212848217807984745591777366372276860411583588494571887934733431113199393}{791913776694483778588698588709929135766318768538930893652343750000000000000} r^{31} + \\
\frac{12891830160861887042312930556116527397598369437831253112410533891470144462896563509}{2375741330083451335766095766129787407298956305616792680957031250000000000000} r^{30} + \\
\frac{1143364706849144471368732701620706675895368660811433194915842968849736588740046217}{169695809291675095411863983294984814807068307544056620068359375000000000000} r^{29} + \\
\frac{1894223361894024164709180344193508276149281595591591986658211519315537547323846207}{237574133008345133576609576612978740729895630561679268095703125000000000000} r^{28} + \\
\frac{21428097029880373218311112435358229670656891082066760972501955864501432138378896531}{2375741330083451335766095766129787407298956305616792680957031250000000000000} r^{27} + \\
\frac{801022019708817904455746198578617530054038040854412364759411591253792343583646439}{81922114830463839164348129866544393355136424331613540722656250000000000000} r^{26} + \\
\frac{6043831092625088541215047733673129681002510108096187925439945057336154334932897427}{593935332520862833941523941532446851824739076404198170239257812500000000000} r^{25} + \\
\frac{6043831092625088541215047733673129681002510108096187925439945057336154334932897427}{593935332520862833941523941532446851824739076404198170239257812500000000000} r^{24} + \\
\frac{801022019708817904455746198578617530054038040854412364759411591253792343583646439}{81922114830463839164348129866544393355136424331613540722656250000000000000} r^{23} + \\
\frac{21428097029880373218311112435358229670656891082066760972501955864501432138378896531}{2375741330083451335766095766129787407298956305616792680957031250000000000000} r^{22} + \\
\frac{1894223361894024164709180344193508276149281595591591986658211519315537547323846207}{237574133008345133576609576612978740729895630561679268095703125000000000000} r^{21} + \\
\frac{1143364706849144471368732701620706675895368660811433194915842968849736588740046217}{169695809291675095411863983294984814807068307544056620068359375000000000000} r^{20} + \\
\frac{12891830160861887042312930556116527397598369437831253112410533891470144462896563509}{2375741330083451335766095766129787407298956305616792680957031250000000000000} r^{19} + \\
\frac{3287151019212848217807984745591777366372276860411583588494571887934733431113199393}{791913776694483778588698588709929135766318768538930893652343750000000000000} r^{18} + \\
\frac{1784422236438075188537138900658095059296529954702208506947548731323074538577597981}{593935332520862833941523941532446851824739076404198170239257812500000000000} r^{17} + \\
\frac{22130456707641639004248146630609315027823814070629995136603247025845612921651603}{1079882422765205152620952620968085185135889229825814854980468750000000000} r^{16} + \\
\frac{41550484881909446388327767743277061617985477251726998056709651669094404010048507}{3167655106777935114354794354839716543065275074155723574609375000000000000} r^{15} + \\
\frac{14904297300954246434065316373615468433612748954602965427264845089050815525174899}{1900593064066761068612876612903829925839165044493434144765625000000000000} r^{14} + \\
\frac{828072648510561263189682099297410898323565661136075420452698337442115035231749}{190059306406676106861287661290382992583916504449343414476562500000000000} r^{13} + \\
\frac{425183741527331139825902027524200329764363303966235727482073723400678572174677}{190059306406676106861287661290382992583916504449343414476562500000000000} r^{12} + \\
\frac{26732729318515826831791274995616579065637953912223549102534868243984792082723}{2534124085422348091483835483871773234452220059324578859687500000000000} r^{11} + \\
\frac{98514958000354677455643814676264534931115549410475725682221654907248284623}{21721063589334412212718589861758056295304743365639247368750000000000} r^{10} + \\
\frac{38291101140138887359782676914615116290259958340221391656013420168256811577}{21721063589334412212718589861758056295304743365639247368750000000000} r^{9} + \\
\frac{10872394332592777284288878621556700840415990768352322461450204898552609}{17731480481089316092015175397353515343105912951542242750000000000} r^{8} + \\
\frac{269061418914533471263783319921967679903930817801083532938975715087}{142748303192765093523448660768454013952468807724850000000000} r^{7} + \\
\frac{6867963997466308046319209185518123663135600673726493180976212363}{13625974395673031654511008527897883150008386191917500000000} r^{6} + \\
\frac{450435638313535005425039251624357069084344950220101681650037}{3921656681119920151743095076056428954738154058375000000} r^{5} + \\
\frac{2068529647022090441678077299141302609199588004130495071}{95388426418240684748995927663275863903634030000000} r^{4} + \\
\frac{161551466808961078632134160985357629261818985772279}{49607330701839093502168550993880180658065000000} r^{3} + \\
\frac{3171065904103137883917151919165713711668601}{8694346127878979529622754612734665450000} r^{2} + \\
\frac{66452121818275070927610813524449}{2453784351049966935520268248500} r + 1
\end{aligned}
$$

$$\Delta'(r) = (r-1)r^9(-\frac{81}{26800}r^{45} -$$
$$\frac{5633195387585655909205183 32973}{6524782699847965260642688600000}r^{44} -$$
$$\frac{1851185129068029582167495838291386131 38971}{150272649123834214092245141454673230000000}r^{43} -$$
$$\frac{11292851072467750513499229152350823090599713979537}{964586985869093484764388491547670179462375000000}r^{42} -$$
$$\frac{279513816459487853798887874632356682945046681528542 07}{33521785350500179520029738666656656731811250000000 0}r^{41} -$$
$$\frac{6082794234920317877806886321199835887018690728961578310225439 1}{12810745158325072495694110581784334585477969924025000000000 0}r^{40} -$$
$$\frac{85629122021009903119059874390413297174632105755690861543660935 23}{3801449378502983468830969770464264501995093249194375000000000}r^{39} -$$
$$\frac{44621655705123136077347662614843260751907658760768760237116789155653}{48712858464531088164876855487234932261279980636105062500000000000}r^{38} -$$
$$\frac{80492686432889156295605195823804626469146709501499514533353144038439997}{246830268060618320599074884792705185173917538245900538281250000000 0}r^{37} -$$
$$\frac{2157246710904829367097195187318479384875565969609496310367800179931386703}{20885638066667704050690951790151977207023791697730045546875000000000}r^{36} -$$
$$\frac{23941595327872587256493987343365062085807713765396772351115918617324986847}{812219258148188490860203680728132446939814121578390660156250000000000}r^{35} -$$
$$\frac{28641097615802981958553267469679468109543713475889363519184564264830177497}{374132492926527769411983585217289355480150599309731130859375000000000}r^{34} -$$
$$\frac{182389272432036105115132679246396634513515042603013756970025287609794539 6887}{10003121389825058255857245331072789083364026549965442867187500000000000}r^{33} -$$
$$\frac{704997006524156214869933487133011461598604208720719906364253572704533642005 47}{175980839265440839686377464157762030170293059675317976367187500000000000}r^{32} -$$
$$\frac{1937320728607288174042845117274152056881858558885139395629838587246738597971278 1}{237574133008345133576609576612978740729895630561679268095703125000000000000}r^{31} -$$
$$\frac{18322970777393752091015565207360611525969701347062569432890666329954781630389608 1}{1187870665041725667883047883064893703649478152808396340478515625000000000000}r^{30} -$$
$$\frac{8069036537776930284141037365943905954467207828990298551287738507372895624224045 9}{2969676662604314169707619707662234259123695382020990851196289062500000000}r^{29} -$$
$$\frac{26511858831944990408878504690774936941328600647969758044518695964422014586538256 9}{593935332520862833941523941532446851824739076404198170239257812500000000 0}r^{28} -$$
$$\frac{2083576048854271631540030942650596651240717984767769603964171153145654174 33}{304331109623322516929120505968381398028364839680590820312500000000 0}r^{27} -$$
$$\frac{19426468826311685890111431991671272181216667262683895205966558507624928619658101}{197978444173620944647174647177482283941579692134732723413085937500000000 0}r^{26} -$$
$$\frac{61747689781078614190389126150275999437373293856272957274583537086839214055846 37}{469514096854437022878675052594819645711256186880789067382812500000000000 0}r^{25} -$$
$$\frac{195942997477312938288591249238312590593933499369727643140885217392697551615218471 1}{1187870665041725667883047883064893703649478152808396340478515625000000000000}r^{24} -$$
$$\frac{20012471149919090534576487714214848267424443570957198256689224909784074027410747}{103293101307976145033308511570860322056476361113773594824218750000000000 0}r^{23} -$$
$$\frac{1101215958042911677780520896365298658454903140870346065371017788516635217436952 93}{5164655065398807251665425578543016102823818055688679741210937500000000000}r^{22} -$$
$$\frac{3266158267899045489938760203475659733691268402291595640652195958330698625969433 61}{1484838331302157084853809853831117129561847691010495425598144531250000000 0}r^{21} -$$
$$\frac{289509871858714149262817301609610759031626458944642575540032303015534612546931}{13606765922585631934513721455497064188424721108916338378906250000000000 0}r^{20} -$$
$$\frac{17630909215964265182870222431299317526595637721076822566564048965898951483251201}{913746665416712052217729140819149002807290886775689492675781250000000000 0}r^{19} -$$
$$\frac{54105352084418197792331252631216415905145343333898279336690202899776497173666487}{3299640736227015744119577452958038065692994868912212056884765625000000000 0}r^{18} -$$
$$\frac{154964968674833837445498705180646917889673008423887717000917031003231609343752063 1}{1187870665041725667883047883064893703649478152808396340478515625000000000000}r^{17} -$$
$$\frac{113542022219360295732060889142809941888436570367304900680632903768183195634437 3}{1170315926149483416633544712379205619359091776165907724609375000000000000}r^{16} -$$
$$\frac{11330668168315445571882115643884537226967185502728708803240987316670851550989}{1683704929826261382380190051260639400787342706422866210937500000000000 0}r^{15} -$$
$$\frac{84578352318555854318068425149237494160595130472327482696493859485784343700267}{194828713308467388532564848788731130662535370314645947265625000000000000 0}r^{14} -$$
$$\frac{51369970419213646121125464421783457092780669359059598876124948621499825163399 31}{197978444173620944647174647177482283941579692134732723413085937500000000 0}r^{13} -$$
$$\frac{21783341529149747877433171520259928464655908499943679551408290728810179477631 37}{152291110902785342036288190136524833801215147795948248779296875000000000 0}r^{12} -$$
$$\frac{39661125052776054791815313579720169806017945409553794150895806492299908416797}{54841674286321591315006827472986782255285233278319313964843750000000000 0}r^{11} -$$
$$\frac{10991026838121001529199524081770600360785491274706023383288186887025132118004 99}{329964073622701574411957745295803806569299486891221205688476562500000000 0}r^{10} -$$
$$\frac{54891046981061400576255703141666268635335458897980274085203832851910572265473 33}{395956888347241889294349294354964567883159384269465446826171875000000000 0}r^{9} -$$
$$\frac{61311068325116029192564527104960721124387188288437966369670406716840091109219 9}{1187870665041725667883047883064893703649478152808396340478515625000000000 0}r^{8} -$$
$$\frac{26894143058737575665255926430243645704851982037548246998334833392541589960819}{15838275533889675571773971774198582715326375370778617873046875000000000 0}r^{7} -$$
$$\frac{16492262328368239775468027331081219825487682371307390093215106720740465996 1}{339391618583350190823727966589969629614136615088113240136718750000000 0}r^{6} -$$
$$\frac{20625289867463619046424933470290161899000367214515775332338073846727247 7}{17404698388889753375575793158459981005853159748108371289062500000000 0}r^{5} -$$
$$\frac{35229105968230339750243342753514011751276304181968500770382355157 9}{14712340142763950444273705121267946750509856084622460937500000 0}r^{4} -$$
$$\frac{29962903292647976025325503049075929992044225870272449515704223}{778430695384336002342524080490367552937029422466796875000 00}r^{3} -$$
$$\frac{23927768287982533616137767221517340691495165213652182978 3}{5184353615613293388894599270665118567679183632812500000 0}r^{2} -$$
$$\frac{34572296001809112450941603979281195831409275758813}{941979478387786606215223136277021659631225585937 5}r -$$
$$\frac{27398732626873500285881217811197978 7}{188694313523723272722484769929687500 0})$$

$$\Delta''(r) = r^{57} + \frac{66452121818275070927610813524449}{2453784351049966935520268248500} r^{56} +$$
$$\frac{3179760250231016863446774673778448377118601}{8694346127878979529622754612734665450000} r^{55} +$$
$$\frac{162894906945201046374046948661769225591462519982279}{49607330701839093502168550993880180658065000000} r^{54} +$$
$$\frac{48378563499458279070496997046791674658021454156922194833}{2193933807619535749226906336255344869783582690000000} r^{53} +$$
$$\frac{231656564107404127657533499876345428450010894244108883079531}{1960828340559960075871547538028214477369077029187500000} r^{52} +$$
$$\frac{7168431160720568553056298409926485056517907420131597702535267113}{13625974395673031654511008527897883150008386191917500000000} r^{51} +$$
$$\frac{285926016781552491757251758712965627095091610902054659627165571887}{142748303192765093523448660768454013952468807724850000000000} r^{50} +$$
$$\frac{11805222279537344870098094733640434340820666060934047270481119207967299}{1773148048108931609201517539735351534310591295154224275000000000} r^{49} +$$
$$\frac{2940817097346045092988068120528287372278483923112119641403310046791028651}{149800438547133877329093723184538319277963747349236188750000000000} r^{48} +$$
$$\frac{18829392186780260998012126575519180137135872634107599504106048177001370983}{3620177264889068702119764976959676049217457227606541228125000000000} r^{47} +$$
$$\frac{47561407068113171420696418508451533053175046368911395678068968300303173325997}{380118612813352213722575322580765985167833008898686828953125000000000} r^{46} +$$
$$\frac{524037357309638139993594284647384667702228606494496816682135156818346707335427}{19005930640667610686128766129038299258391650444934341447656250000000000} r^{45} +$$
$$\frac{8459313447387326074946974058059972437796587091359021440657895512613663035609}{150840719370377862588323540706653168717394051150272551171875000000000} r^{44} +$$
$$\frac{2877751246306348895664871808710298879269877759533231616327271370672552413629167}{27151329486668015265898237327197570369130929207049059210937500000000000} r^{43} +$$
$$\frac{2578756730434961337682727762586159353112520159903506447727051475200597178416409}{13772413507730152671107801542781376274196848148503145976562500000000000} r^{42} +$$
$$\frac{492369024007770206158782745957266597900056372641367109988420049606172193809987419}{1583827553388967557177397177419858271532637537077861787304687500000000000} r^{41} +$$
$$\frac{827254739411915971204146165247084942401593952605011862683522913598100754467256291}{1696958092916750954118639832949848148070683075440566200683593750000000000} r^{40} +$$
$$\frac{8616210554080518945933099499459364853363012529112111429131028867463619051637282857}{118787066504172566788304788306489370364947815280839634047851562500000000000} r^{39} +$$
$$\frac{24431515620756683731121214566700356307778212944866802042856090003534524137775807833}{2375741330083451335766095766129787407298956305616792680957031250000000000000} r^{38} +$$
$$\frac{5521962711456028760426891066551076472363379779569429960353154893961457922388134417}{395956888347241889294349294354964567883159384269465446826171875000000000000} r^{37} +$$
$$\frac{21561564951167919750832487402775766820265336541427813068300970403451271092619370889}{1187870665041725667883047883064893703649478152808396340478515625000000000000} r^{36} +$$
$$\frac{18009464540569127285363360433419812697543905209841848691756097691339777152496452261}{7919137766944837785886985887099291357663187685389308936523437500000000000000} r^{35} +$$
$$\frac{65317677663253357151894511940209678389193319191213490439059004031459876355124802259}{2375741330083451335766095766129787407298956305616792680957031250000000000000} r^{34} +$$
$$\frac{6361723402465704601391008974020835271870013536882077258218330638936049738047840343}{197978444173620944647174647177482283941579692134732723413085937500000000000} r^{33} +$$
$$\frac{3322181371831173186062696934390631441994401878066104511021752322523938976696259767}{91374666541671205221772914081914900280729088677568949267578125000000000000} r^{32} +$$
$$\frac{4117461692411435385433658921230255753386348979644534206373486498604632172945064269}{103293101307976145033308511570860322056476361113773594824218750000000000000} r^{31} +$$
$$\frac{100667123751738575301792677126882266925325220092976644231277321324831547378171258549}{23757413300834513357660957661297874072989563056167926809570312500000000000000} r^{30} +$$
$$\frac{58239281417937548181056119188246707626409658757859402832597412456373577529537229}{1333188176253339694593768667861833561896159542994833154296875000000000000} r^{29} +$$
$$\frac{58239281417937548181056119188246707626409658757859402832597412456373577529537229}{1333188176253339694593768667861833561896159542994833154296875000000000000} r^{28} +$$
$$\frac{100667123751738575301792677126882266925325220092976644231277321324831547378171258549}{23757413300834513357660957661297874072989563056167926809570312500000000000000} r^{27} +$$
$$\frac{4117461692411435385433658921230255753386348979644534206373486498604632172945064269}{103293101307976145033308511570860322056476361113773594824218750000000000000} r^{26} +$$
$$\frac{3322181371831173186062696934390631441994401878066104511021752322523938976696259767}{91374666541671205221772914081914900280729088677568949267578125000000000000} r^{25} +$$
$$\frac{6361723402465704601391008974020835271870013536882077258218330638936049738047840343}{197978444173620944647174647177482283941579692134732723413085937500000000000} r^{24} +$$
$$\frac{65317677663253357151894511940209678389193319191213490439059004031459876355124802259}{2375741330083451335766095766129787407298956305616792680957031250000000000000} r^{23} +$$
$$\frac{18009464540569127285363360433419812697543905209841848691756097691339777152496452261}{7919137766944837785886985887099291357663187685389308936523437500000000000000} r^{22} +$$
$$\frac{21561564951167919750832487402775766820265336541427813068300970403451271092619370889}{1187870665041725667883047883064893703649478152808396340478515625000000000000} r^{21} +$$
$$\frac{5521962711456028760426891066551076472363379779569429960353154893961457922388134417}{395956888347241889294349294354964567883159384269465446826171875000000000000} r^{20} +$$
$$\frac{24431515620756683731121214566700356307778212944866802042856090003534524137775807833}{2375741330083451335766095766129787407298956305616792680957031250000000000000} r^{19} +$$
$$\frac{8616210554080518945933099499459364853363012529112111429131028867463619051637282857}{118787066504172566788304788306489370364947815280839634047851562500000000000} r^{18} +$$
$$\frac{827254739411915971204146165247084942401593952605011862683522913598100754467256291}{1696958092916750954118639832949848148070683075440566200683593750000000000} r^{17} +$$
$$\frac{492369024007770206158782745957266597900056372641367109988420049606172193809987419}{1583827553388967557177397177419858271532637537077861787304687500000000000} r^{16} +$$
$$\frac{2578756730434961337682727762586159353112520159903506447727051475200597178416409}{13772413507730152671107801542781376274196848148503145976562500000000000} r^{15} +$$
$$\frac{2877751246306348895664871808710298879269877759533231616327271370672552413629167}{27151329486668015265898237327197570369130929207049059210937500000000000} r^{14} +$$
$$\frac{8459313447387326074946974058059972437796587091359021440657895512613663035609}{150840719370377862588323540706653168717394051150272551171875000000000} r^{13} +$$
$$\frac{524037357309638139993594284647384667702228606494496816682135156818346707335427}{19005930640667610686128766129038299258391650444934341447656250000000000} r^{12} +$$
$$\frac{47561407068113171420696418508451533053175046368911395678068968300303173325997}{380118612813352213722575322580765985167833008898686828953125000000000} r^{11} +$$
$$\frac{18829392186780260998012126575519180137135872634107599504106048177001370983}{3620177264889068702119764976959676049217457227606541228125000000000} r^{10} +$$
$$\frac{2940817097346045092988068120528287372278483923112119641403310046791028651}{149800438547133877329093723184538319277963747349236188750000000000} r^{9} +$$

$$\frac{118052222795373448700980947336404343408206660609340472704811192079672 99}{17731480481089316092015175397353515343105912951542242750000000000}r^8 +$$
$$\frac{2859260167815524917572517587129656270950916109020546596271655718 87}{142748303192765093523448660768454013952468807724850000000000}r^7 +$$
$$\frac{716843116072056855305629840992648505651790742013159770253526711 3}{1362597439567303165451100852789788315000838619191750000000 0}r^6 +$$
$$\frac{23165656410740412765753349987634542845001089424410888307953 1}{196082834055996007587154753802821447736907702918750000 0}r^5 +$$
$$\frac{48378563499458279070496997046791674658021454156922194833}{2193933807619535749226906336255344869783582690000000}r^4 +$$
$$\frac{162894906945201046374046948661769225591462519982279}{4960733070183909350216855099388018065806500000 0}r^3 +$$
$$\frac{317976025023101686344677467377844837711860 1}{869434612787897952962275461273466545000 0}r^2 +$$
$$\frac{6645212181827507092761081352444 9}{2453784351049966935520268248500}r + 1$$
